# Supplementary material for: Visually Grounded Concept Composition
Source: arXiv:2109.14115 source file (2021-09-29)
Supplement: Supplementary file 1 [file supp_flops_vs_composition_times.tex]

%!TEX root = main.tex

\begin{table}[t]
    \centering
    \small
    \vspace{-1em}
    {
        \tabcolsep 2.5pt
	    \begin{tabular}{l@{\;} cccccc@{\;}}
	        \addlinespace
	        \toprule
	        {\# of Compositions} & &  2 & 3 & 4 & 5 \\
	        \midrule
	        {FLOPS} & &  38.37G & 38.40G & 38.44G & 38.47G\\
	        \bottomrule
	    \end{tabular}
	}
    \caption{FLOPS of \ourmethod under different number of compositions (The FLOPS calculate the FLOPS using the model with 6 layers of PT and 5 layers of CT)}
    \label{tab:supp_complexity_vs_num_composition}
\end{table}
